# Supplementary material for: DecompOpt: Controllable and Decomposed Diffusion Models for Structure-based Molecular Optimization
Source: arXiv:2403.13829 source file (2024-03-07)

# Controllable and Decomposed Diffusion Model

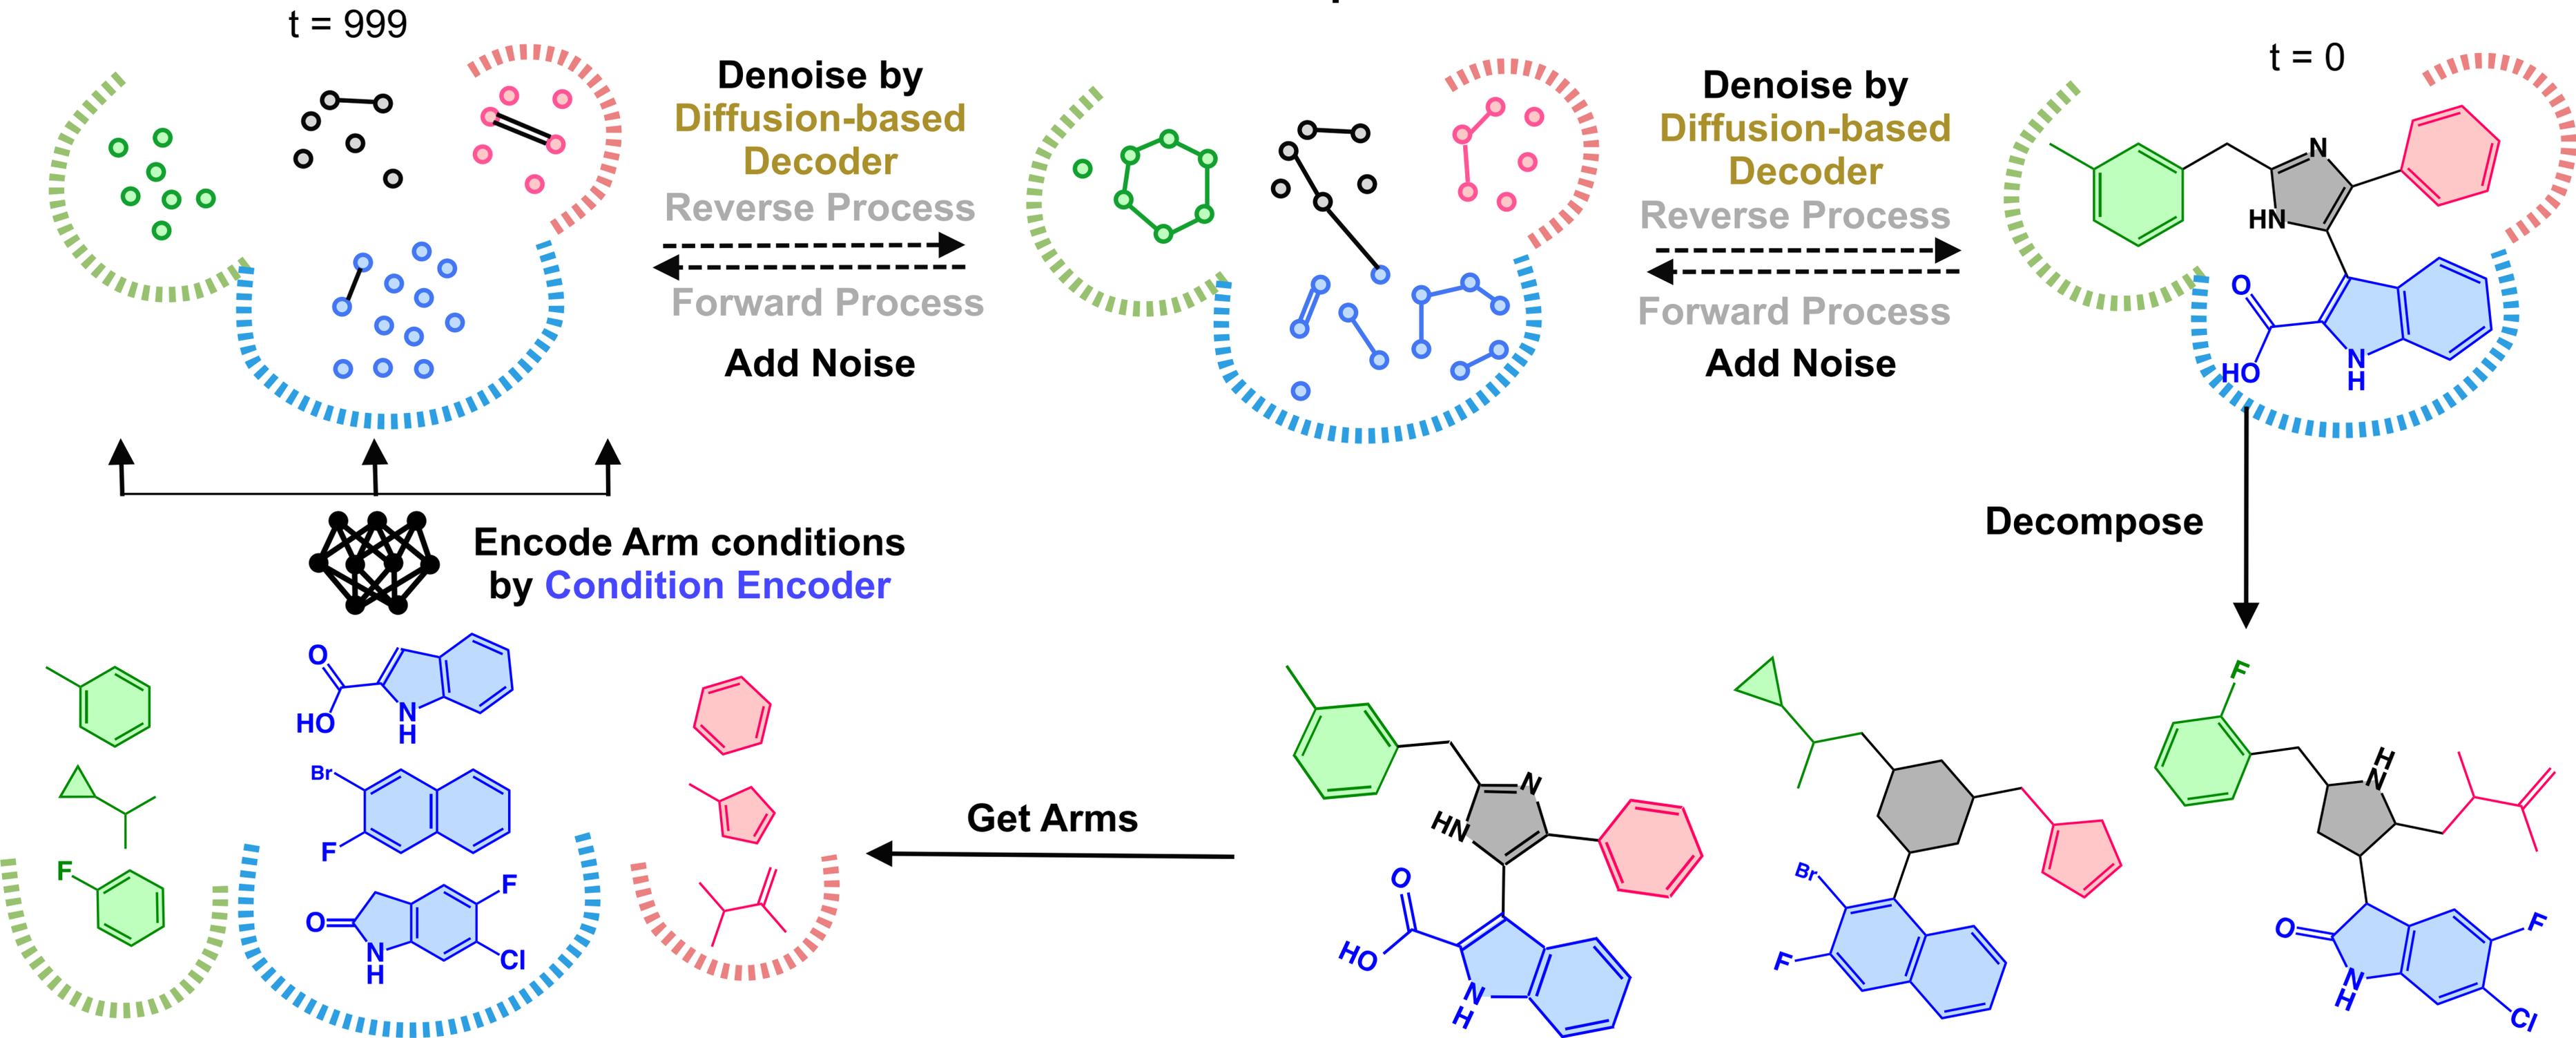

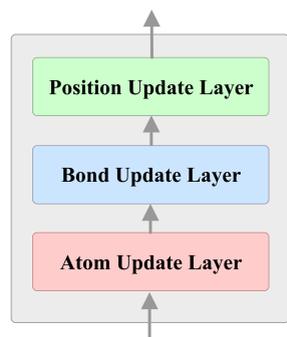

(a) SE(3)-equivariant Layer

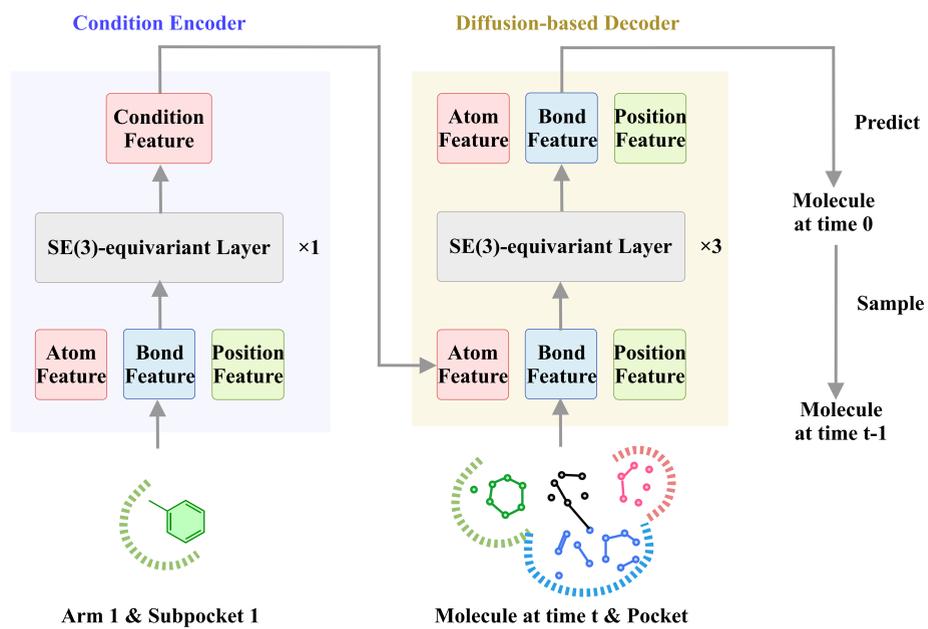

(b) Denoising one step (sampling)

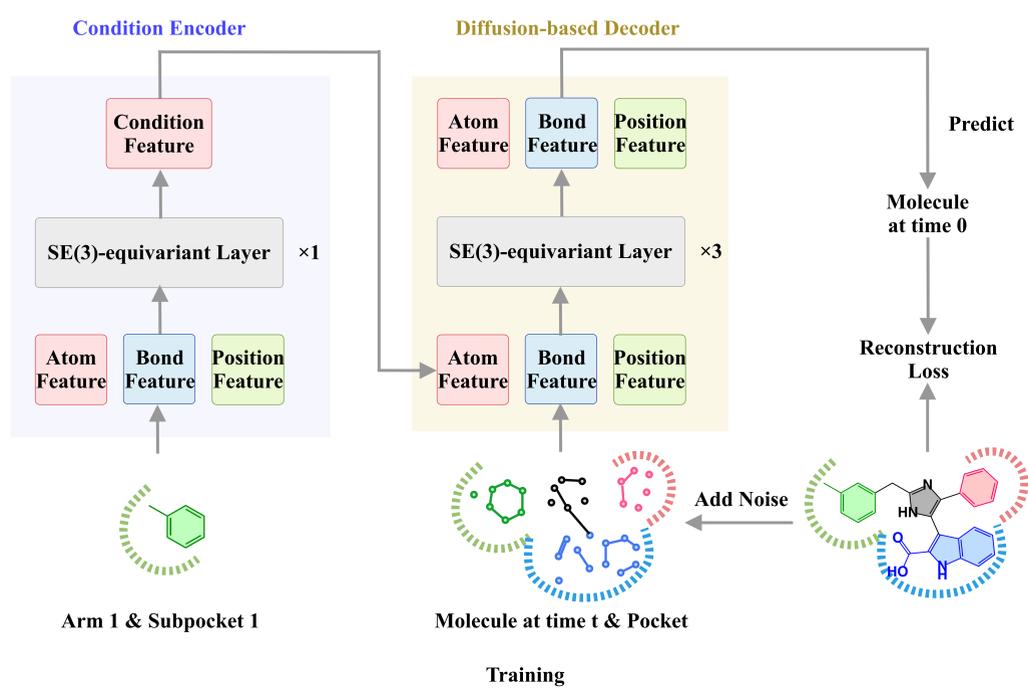

Training

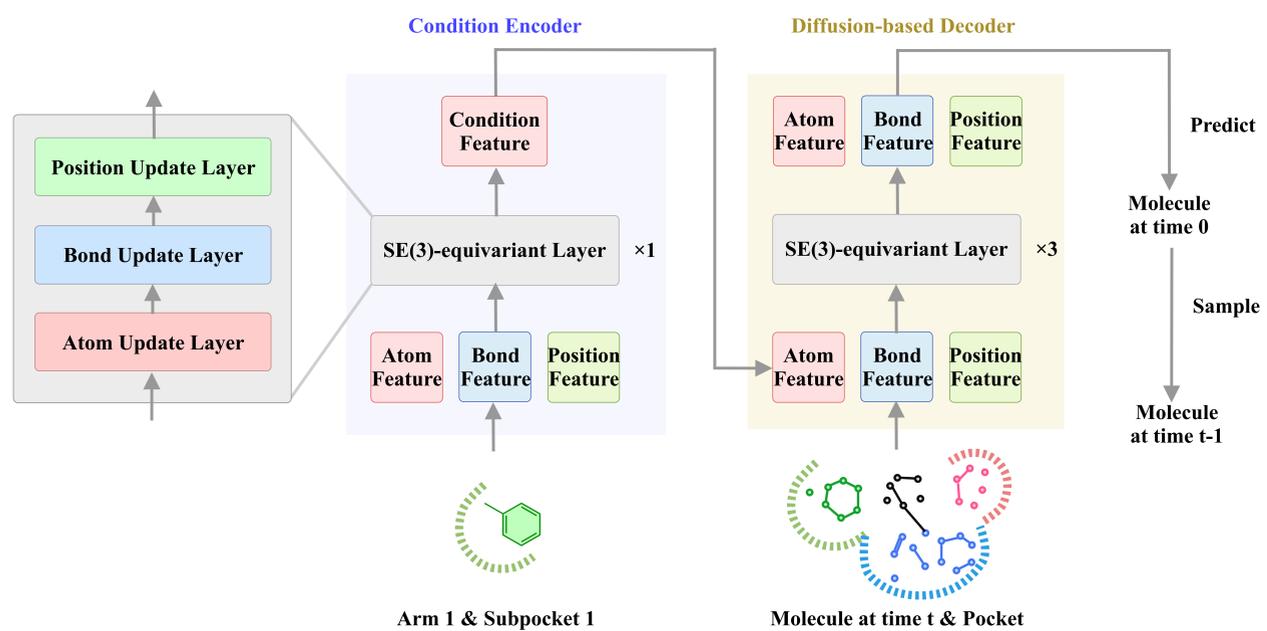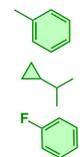

Supplement: Supplementary file 1 [file Overall_framework_appendix.pdf]
